# Supplementary material for: Cellular automata as convolutional neural networks
Source: arXiv:1809.02942 source file (2020-01-16)
Supplement: Supplementary file 1 [file wgilpin_ca_supps.pdf]

# Supplementary material for "Cellular automata as convolutional neural networks"

July 23, 2019

# Contents


**1 Train vs. test performance** **3**

**2 Experiments with alternate networks and parameters** **3**

**3 Dynamics of training deep networks on cellular automata** **4**

**4 Symbol distributions in trained networks** **8**

**5 Mutual information and layer specialization** **9**

# 1 Train vs. test performance

As described in the main text, for all networks, separate random training and testing image sets were generated using the CA rule being studied. Additionally, a separate validation data set was used to determine when to stop training. In earlier stages of experiments, during which hyperparameters were being optimized, separate validation datasets with separate CA dynamical rules were used as well.

We observe that, during training, overfitting to the input data set was minimal. The training and testing performance were nearly identical throughout training (Figure S1), which is a consequence of the network learning the full rule table for the CA—at which point the network has little possible improvement in accuracy.

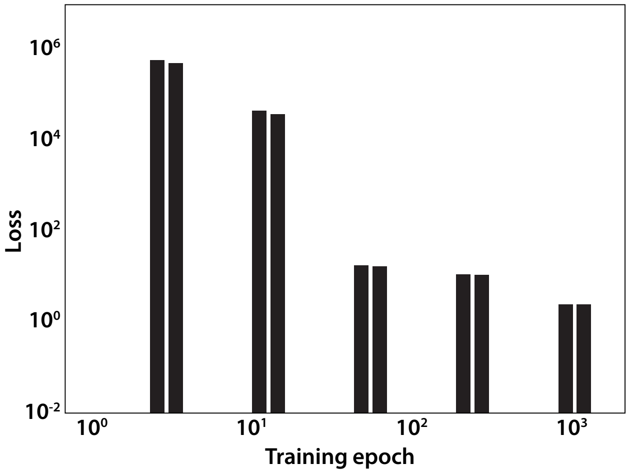


**Figure S1** The performance on the train (left) and test (right) image sets at different training epochs.

# 2 Experiments with alternate networks and parameters

In order to determine the degree to which results in the main text depended on hyperparameters of the networks, we trained an alternative set of networks using different optimizers, loss functions, and network shapes. As described in the main text, and shown in Figures S2

and S3, all reported results are nearly identical.

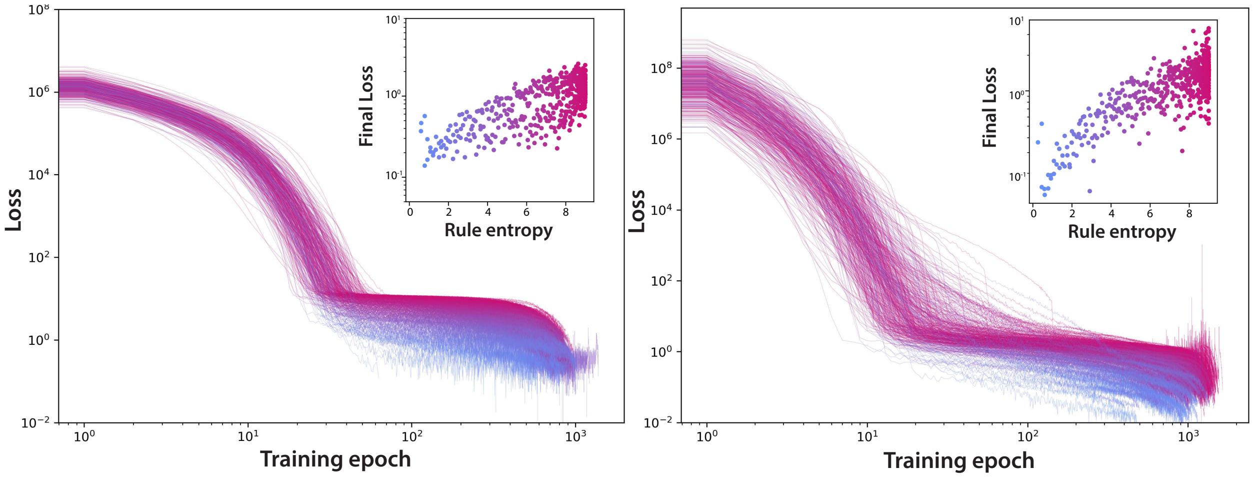


**Figure S2** The loss versus time during training for two alternative networks, colored by the rule entropy $\mathcal{H}_{ca}$. Left panel corresponds to the "large" network that has the same hyperparameters, loss function, and optimizer as the network used in the main text, but double the number of layers and double the number of neurons. Right panel corresponds to a network with the same depth and neuron count as the main text, but which was trained using a different optimizer (SGD), different loss (cross entropy), and with different hyperparameters. As in Figure 2 in the main text, both panels show 512 networks trained on randomly-chosen cellular automata. The entropy of the resulting rule table is characteristic of the CA, and it is indicated by $\mathcal{H}_{ca} = 0$ (blue, minimum entropy CA) to $\mathcal{H}_{ca} = 9$ (magenta, maximum entropy CA). The inset panels final loss for each network at the end of training, shown as a function of $\mathcal{H}_{ca}$.

# 3 Dynamics of training deep networks on cellular automata

In order to study the dynamics of training in more detail, ten replicate networks (with different random initial weights) were trained using the Game of Life cellular automata, as well as four other randomly-generated CA. Networks had the same shape and training parameters as those described in the main text. Over the roughly 1500 training steps. the network was periodically analyzed in order to determine the growth in its discrimination power over time. Because sampling and analyzing the network mid-training introduces computational expenses, for the analysis here the network was inspected at 40 logarithmically-spaced in-

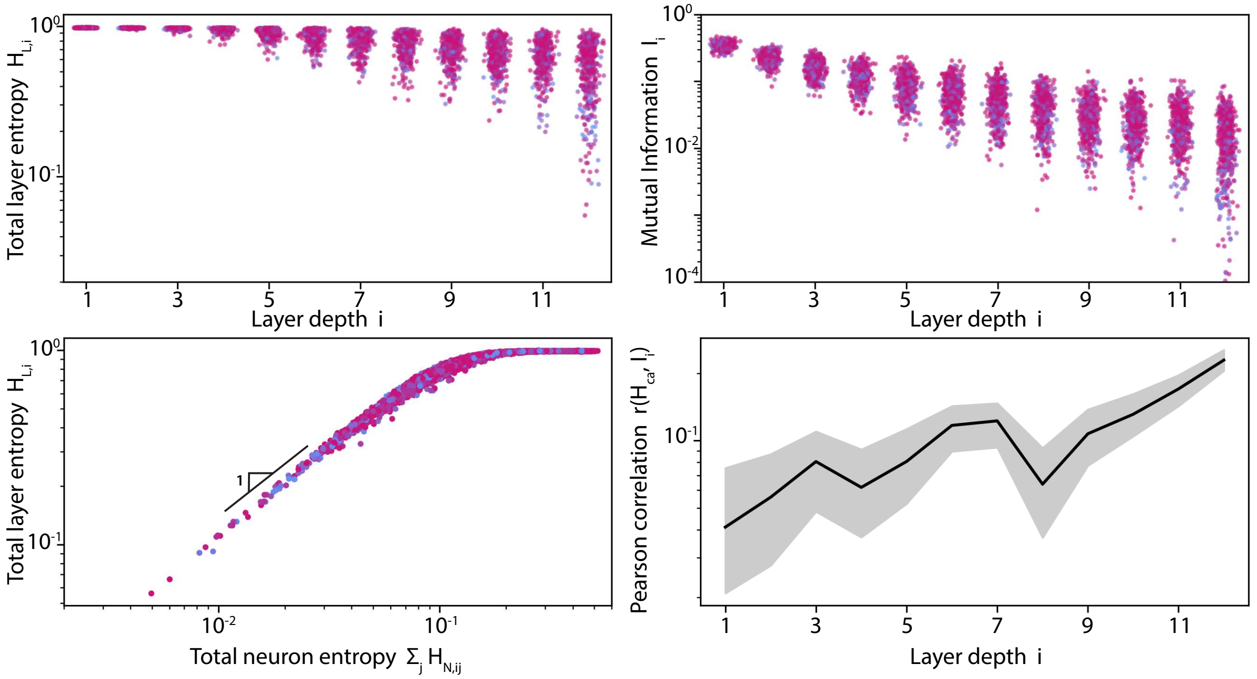


**Figure S3 Internal representations of cellular automata in the alternative network.** (A) The individual layerwise entropy ($\mathcal{H}_{L,i}/D$) for the 2560 networks ($5$ replicates for each of the $512$ possible values of $\lambda$. Noise has been added to the horizontal coordinates (layer index) to facilitate visualization. Coloration corresponds to the entropy $\mathcal{H}_{ca}$ of the underlying CA. which runs from blue (a null automaton that maps all inputs to zero or one) to red (an automaton that maps an equal number of input cases to $0$ or $1$). (B) The normalized mutual information ($\mathcal{I}_i$) as a function of layer index $i$. Random noise has been added to the layer index in this panel as well. (C) The normalized layerwise entropy ($\mathcal{H}_{L,i}/D$) versus the normalized total layerwise neuron entropy ($\mathcal{H}_{N,ij}/N$), with the linear scaling annotated. (D) The Pearson correlation coefficient $r$ between the rule entropy $\mathcal{H}_{ca}$ and the mutual information ($\mathcal{I}_i$). Error range corresponds to bootstrapped 25% -75% quantiles.

tervals, in order to allow more sampling at earlier stages of training. For all accuracy figures reported below, unseen test/validation data consisting of random-generated binary images were used.

During the first $\sim 10$ training epochs, the total loss decreases monotonically and nearly identically across all CA (Figure S4A). However, when the predictions of the network are rounded to the nearest integer and then compared on a case-by-case basis to the correct values, it is clear that during these early stages of training zero input $\sigma$ are correctly classified. Inspection of the network's output values confirms that this occurs because, during early stages of training, the system consistently produces values that are too small or too large to be sensitive to the input data—resulting in all transitions $\sigma \to m$ being either too large or too small, and thus misclassifying all inputs. Consistent with the network acclimating and scaling to the input domain, during this period there is a corresponding increase in the number of unique activations observed in each layer—which measures the amount that layers discriminate distinct inputs (Figure S4C). This period of training ends when the last layers of the network approach a point at which the number of unique activation patterns is nearly unique for every input $\sigma$.

The next stage of training consists of the network learning individual rules, as shown by the rapid ascent in the number of input cases correctly classified in Figure S4B. During this period of training, different rules are grouped together and consolidated in different ways, leading to a decrease in the number of unique activations per layer (Figure S4C). During this period, the network begins cause different input cases to "coalesce," in which multiple input cases $\sigma$ (that map to the same output symbol $m$) get merged together into a single activation pattern at some layer of the network—causing the two inputs to become indistinguishable in that layer, and all later layers. This coalescence process is indicative of the networks implementing the CA rules in a manner analogous to the layerwise tree search described in the main text. Due to the hierarchical structure of this manner of representing the network, a decrease in number of unique activation patterns is more prominent in deeper layers of the

network (lower panels of Figure S4C). As explored further in Section 4, the degree to which the number unique activations decreases is set by the CA ruleset $\mathcal{H}_{ca}$—lower $\mathcal{H}_{ca}$ CA are more "compressible," and so the decrease in the number of unique activations is much more pronounced in these networks.

One minor event that occurs during the final stages of training can be observed in earlier layers, where the number of unique symbols increases very slightly, increasing the discrimination power of the network in earlier layers. This may be the result of later layers "saturating" the amount of cases that they can individually distinguish, causing input cases to be consolidated at earlier stages. This may also explain the smooth appearance of $\mathcal{H}_{L,i}$ vs. $i$ in the fully-trained networks, which suggests that—across the layers—the network interpolates between the entropy of the input ($\mathcal{H} = 9$)and that of the output (which is determined by the CA ruleset and $\mathcal{H}_{ca}$).

In summary, training large networks on cellular automata involves a transient in which the scale and value ranges of the network are set, followed by a specialization phase in which specific input cases $\sigma$ are mapped to their respective output symbols $m$. These mappings initially occur in the last layers of the network, but as training progresses input cases that produce the same output symbol coalesce to the same activation pattern in progressively earlier layers of the network. This occurs because when two input cases produce the same activation in an early layer, they produce the same activation pattern in all later layers—making it impossible for them to be distinguished again in later layers during subsequent stages of training. This irreversibility when two input symbols coalesce to the same representation is responsible for differentiation across layers, and it appears that this process occurs more slowly when there is a more even distribution of output symbols—and thus when $\mathcal{H}_{ca}$ is maximal.

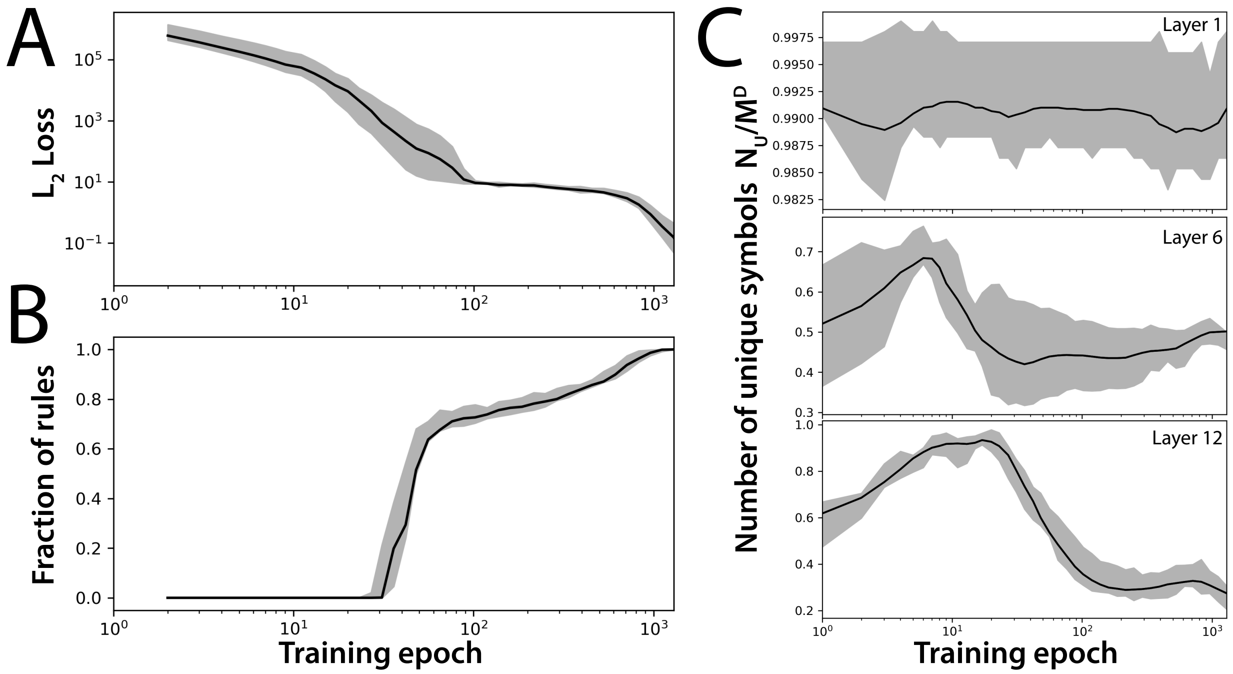


**Figure S4 Training stages of neural networks.** (A) The loss versus time during training. (B) The fraction of input cases $\sigma$ assigned to correct output states $m$. (C) The number of unique activation symbols in each layer as a function of training epoch, for three representative depths in the network. In all panels, gray range corresponds to a 25%-75% quantiles across 15 replicate networks.

# 4 Symbol distributions in trained networks

Figure S5 shows rank-frequency plots for different activation patterns as a function of layer index and $\mathcal{H}_{ca}$, generated for a set of random binary test data that was not used during training. Flatter and wider curves correspond to more uniform activation pattern distributions, such as cases in which a layer exhibits a different activation pattern for each of the uniformly-distributed 512 input cases. Two trends are apparent in the plots: later layers tend to show a narrower distribution of activation patterns, and larger $\mathcal{H}_{ca}$ CA consistently generate networks with broader activation symbol distributions across all layers. The change in the distribution of unique activation symbols across layers is consistent with the structure of the network, because the training data consists of a uniform distribution over the 512 possible input $\sigma$. Because many different $\sigma$ map to the same output symbol $m$, the representations of different input symbols that map to the same output (i.e., $\sigma_1 \rightarrow m$, $\sigma_2 \rightarrow m$

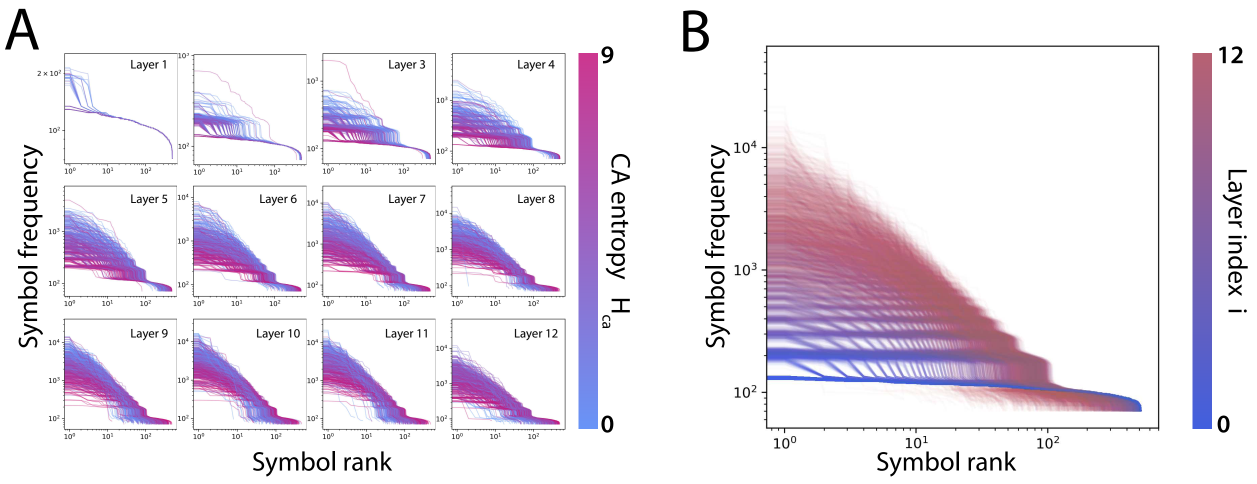


**Figure S5 Rank-frequency distributions across trained networks.** (A) The rank frequency plots for each layer, colored by the CA ruleset ($\mathcal{H}_{ca}$). (B) The rank-frequency distributions across all layers, colored by the layer index.

for $\sigma_1 \neq \sigma_2$ under the CA rule table) can be merged into the same activation pattern any point before the final layer.

That the the symbol distribution narrows gradually across layers—as opposed to abruptly at the first or last hidden layer—indicates that the network is performing something analogous to a layerwise tree search, in which inputs that map to the same output are mapped onto the same activation symbol at some point before the final layer. Inspection of activation pattern distributions confirms that when two input symbols coalesce to the same activation pattern, they appear as the same activation pattern in all subsequent layers. Moreover, the general dependence of the symbol distributions on the CA ruleset, and thus $\mathcal{H}_{ca}$, indicates that more complicated rule tables are more irreducible during training; the network is not able to narrow down the input distribution as quickly, leading to a shallower decrease in activation symbol entropy across layers.

# 5 Mutual information and layer specialization

We define a measure of layer specialization in the form of the total correlation, or the mutual information between a given layer's activation patterns, and the firing patterns of its

constituent neurons

$$\mathcal{I}_i = \sum_j \mathcal{H}_{N,ij} - \mathcal{H}_{L,i}. \tag{A1}$$

Here, the maximum value of of this quantity is $\mathcal{I}^{max} = n - \log_2(M^D)$, where $n$ is the total number of neurons. This case corresponds to one in which each neuron fires essentially randomly with probability 1/2, in which case $\mathcal{H}_{N,ij} = 1$ for all $ij$. In this case, there will be a unique layer activation pattern for every input case, and so $\mathcal{H}_{L,i} = D$ for all $i$.

We show Eq. S6 for the networks studied in the main text in Figure S6A. We find that the total correlation decreases across layers, suggesting that the firing patterns of layers become more independent from their constituent neurons at deeper levels of the network—consistent with deeper network layers learning generic features of the input data that require multiple neurons to jointly represent.[1] The last two layers have higher total correlation than the earlier layers, due to these layers primarily being used to consolidate inputs into the two output cases, 0 and 1. A relationship between $\mathcal{I}_i$ and $\mathcal{H}_{ca}$ can be seen in the Figure as color gradation in the final layer of the network. Explicit calculation of the Pearson correlation confirms that this pattern emerges in several of the late layers (Figure S6B); however it is much more pronounced in the last layer.

In principle, additional the total correlations could also be calculated for the total network versus individual neurons, or for the total network versus single layers—however, these cases provide little additional information here because $\mathcal{H}_T \approx M^D$ for our trained networks.

# References


[1] Vergara, J. R. & Estévez, P. A. A review of feature selection methods based on mutual information. *Neural computing and applications* **24**, 175–186 (2014).

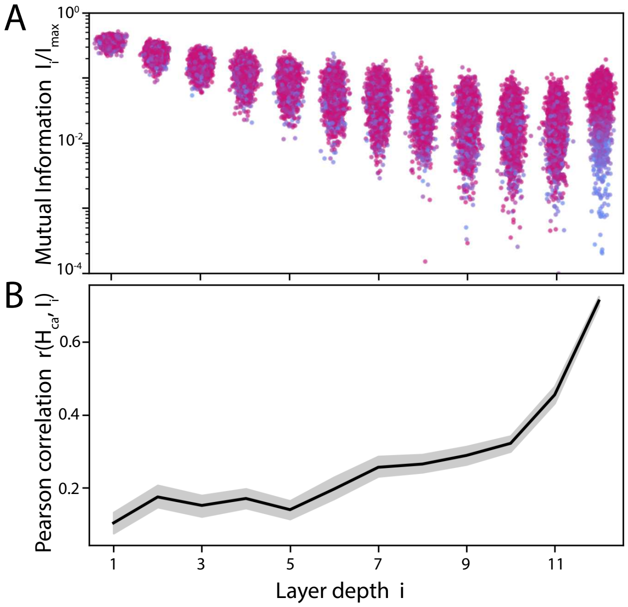


**Figure S6 Layer specialization in neural networks trained on cellular automata.** (A) The normalized mutual information $\mathcal{I}_i$ as a function of layer index $i$, normalized by its maximum possible value $\mathcal{I}_{max} = 100 - 9$. Random noise has been added to the horizontal coordinates (layer index) to facilitate visualization. As in previous figures, coloration corresponds to the entropy $\mathcal{H}_{ca}$ of the underlying CA. (B) The Pearson correlation coefficient $r$ between the rule entropy $\mathcal{H}_{ca}$ and the mutual information ($\mathcal{I}_i$). Error range corresponds to bootstrapped 25% -75% quantiles.
